# Supplementary material for: Multi-modal Domain Adaptation for REG via Relation Transfer
Source: arXiv:2309.13247 source file (2023-09-23)
Supplement: Supplementary file 2 [file suppl_cp.tex]

\appendix

% --- PDF will be split by an editor (e.g. macOS preview), so need to restart from page 1
\setcounter{page}{1}

% --- repeat the title (AT: haven't found a more elegant way to do this...)
\twocolumn[
\centering
\Large
\textbf{Multi-modal Domain Adaptation for REG via Relation Transfer} \\
\vspace{0.5em}Supplementary Material \\
\vspace{1.0em}
] %< twocolumn
\appendix

\section{Performance on Different Source Datasets}
In the main submission, we use RefCOCO as the source dataset and test its transferring performance on RefCOCO+, RefCOCOg and RefClef. We pre-train on RefCOCO since it has the most number of expressions, and differs from other REG datasets. In this section, we test the performance of switching the source and target datasets. Table~\ref{tab:suppl-swith} shows the transferring performance of using RefCOCO+ as the source dataset and RefCOCOg as the target dataset. The results show that our proposed approach achieved consistent improvements while using different source datasets. 

% Please add the following required packages to your document preamble:
% \usepackage[table,xcdraw]{xcolor}
% If you use beamer only pass "xcolor=table" option, i.e. \documentclass[xcolor=table]{beamer}
\begin{table}[h]
\centering
\caption{Performance comparison transferring from RefCOCO+ to RefCOCOg (Best results are \textbf{bolded})}
\label{tab:suppl-swith}
\begin{tabular}{l|cc}
\toprule
RefCOCO+ $\xrightarrow[]{}$ RefCOCOg   & Val   & Test  \\
\midrule\midrule
Train on target    & 67.63 & 67.44 \\
Vanilla finetune on target & 71.32 & 70.05 \\
DANN - Language~\cite{ganin2015unsupervised}          & 72.37 & 72.41 \\
DANN - Visual~\cite{ganin2015unsupervised}        & 71.77 & 71.08 \\
DANN - Language\&Visual~\cite{ganin2015unsupervised}          & 70.81 & 70.31 \\
Adversarial-cat \cite{tzeng2017adversarial}     &       &  \\
CDAN\cite{long2017conditional}               & 72.37 & 73.00    \\
SRDA\cite{cai2019learning}              & 72.65 & 71.13 \\
Ours               &  \textbf{74.69}     &   \textbf{74.12}   \\
\bottomrule
\end{tabular}
\end{table}

\begin{table}[h]
\centering
\caption{Performance comparison transferring from RefCOCOg to RefCOCO (Best results are \textbf{bolded})}
\label{tab:suppl-swith1}
\begin{tabular}{l|cc}
\toprule
RefCOCO+ $\xrightarrow[]{}$ RefCOCOg   & Val   & Test  \\
\midrule\midrule
Train on target    & 67.63 & 67.44 \\
Vanilla finetune on target & 71.32 & 70.05 \\
DANN - Language~\cite{ganin2015unsupervised}          & 72.37 & 72.41 \\
DANN - Visual~\cite{ganin2015unsupervised}        & 71.77 & 71.08 \\
DANN - Language\&Visual~\cite{ganin2015unsupervised}          & 70.81 & 70.31 \\
Adversarial-cat \cite{tzeng2017adversarial}     &       &  \\
CDAN\cite{long2017conditional}               & 72.37 & 73.00    \\
SRDA\cite{cai2019learning}              & 72.65 & 71.13 \\
Ours               &  \textbf{74.69}     &   \textbf{74.12}   \\
\bottomrule
\end{tabular}
\end{table}

\section{Convergence Comparison }

A merit of our approach is that it does not require  extra modification on the target network, therefore, less adaptation is needed for fine-tuning. In this section, we compare the validation accuracy of the proposed approach with baselines during the fine-tuning. % First, we list the performance of each methods while directly test on the target datasets. Table~\ref{} to Table~\ref{} show the results. Secondly, we draw  
The performances are recorded every 2000 iterations of the first 20000 iterations in fine-tuning for better visualization. Figure~\ref{fig:refcocoplus} to   Figure~\ref{fig:refclef} demonstrate the comparison. 
% Besides, we also list the initial test performance on target task for each method, showing in Table~\ref{} to Table~\ref{}. 

We find that the proposed approach not only has the best final performance, but also achieves better performance than the baseline models at the initial stage where we have not conducted fine-tuning but directly test the pre-trained model on target datasets. 

\begin{figure}[t]
\begin{center}
% \fbox{\rule{0pt}{2in} \rule{0.9\linewidth}{0pt}}
   \includegraphics[width=0.95\linewidth]{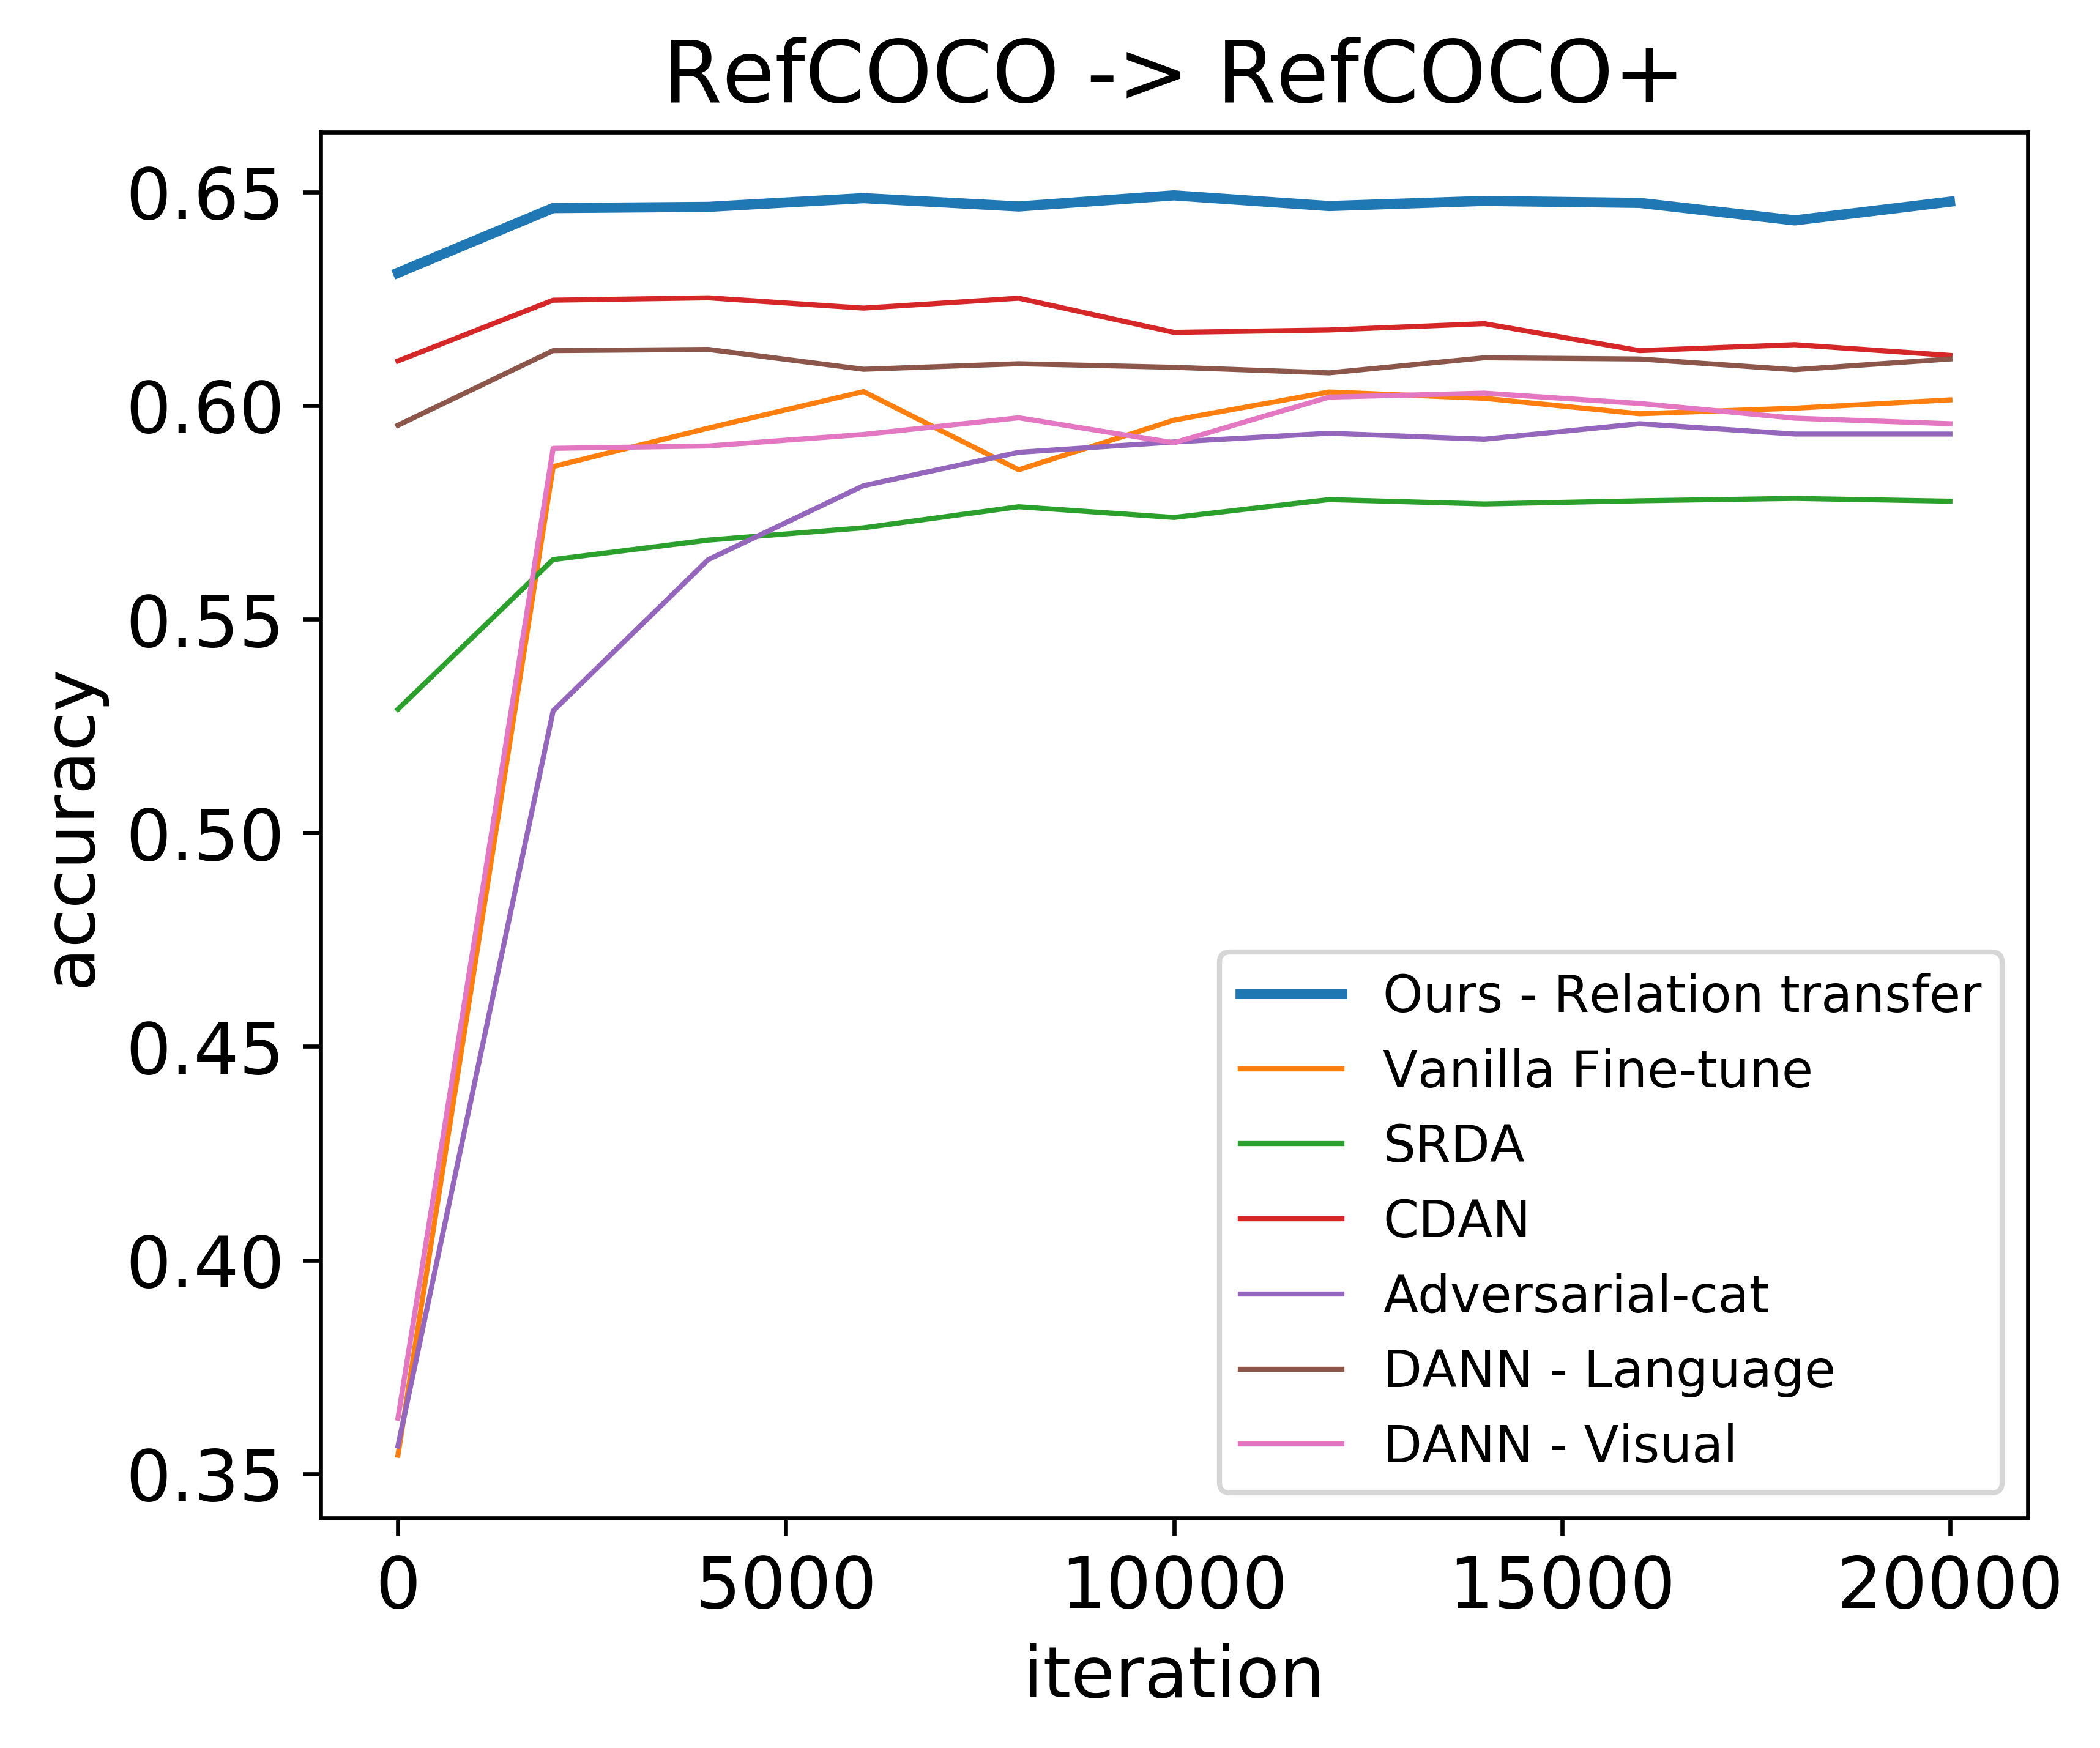}
\end{center}
   \caption{Convergence comparison of the proposed approach with baseline models for domain adaptation  from RefCOCO to RefCOCO+ }
\label{fig:refcocoplus}
\end{figure}

\begin{figure}[t]
\begin{center}
% \fbox{\rule{0pt}{2in} \rule{0.9\linewidth}{0pt}}
   \includegraphics[width=0.95\linewidth]{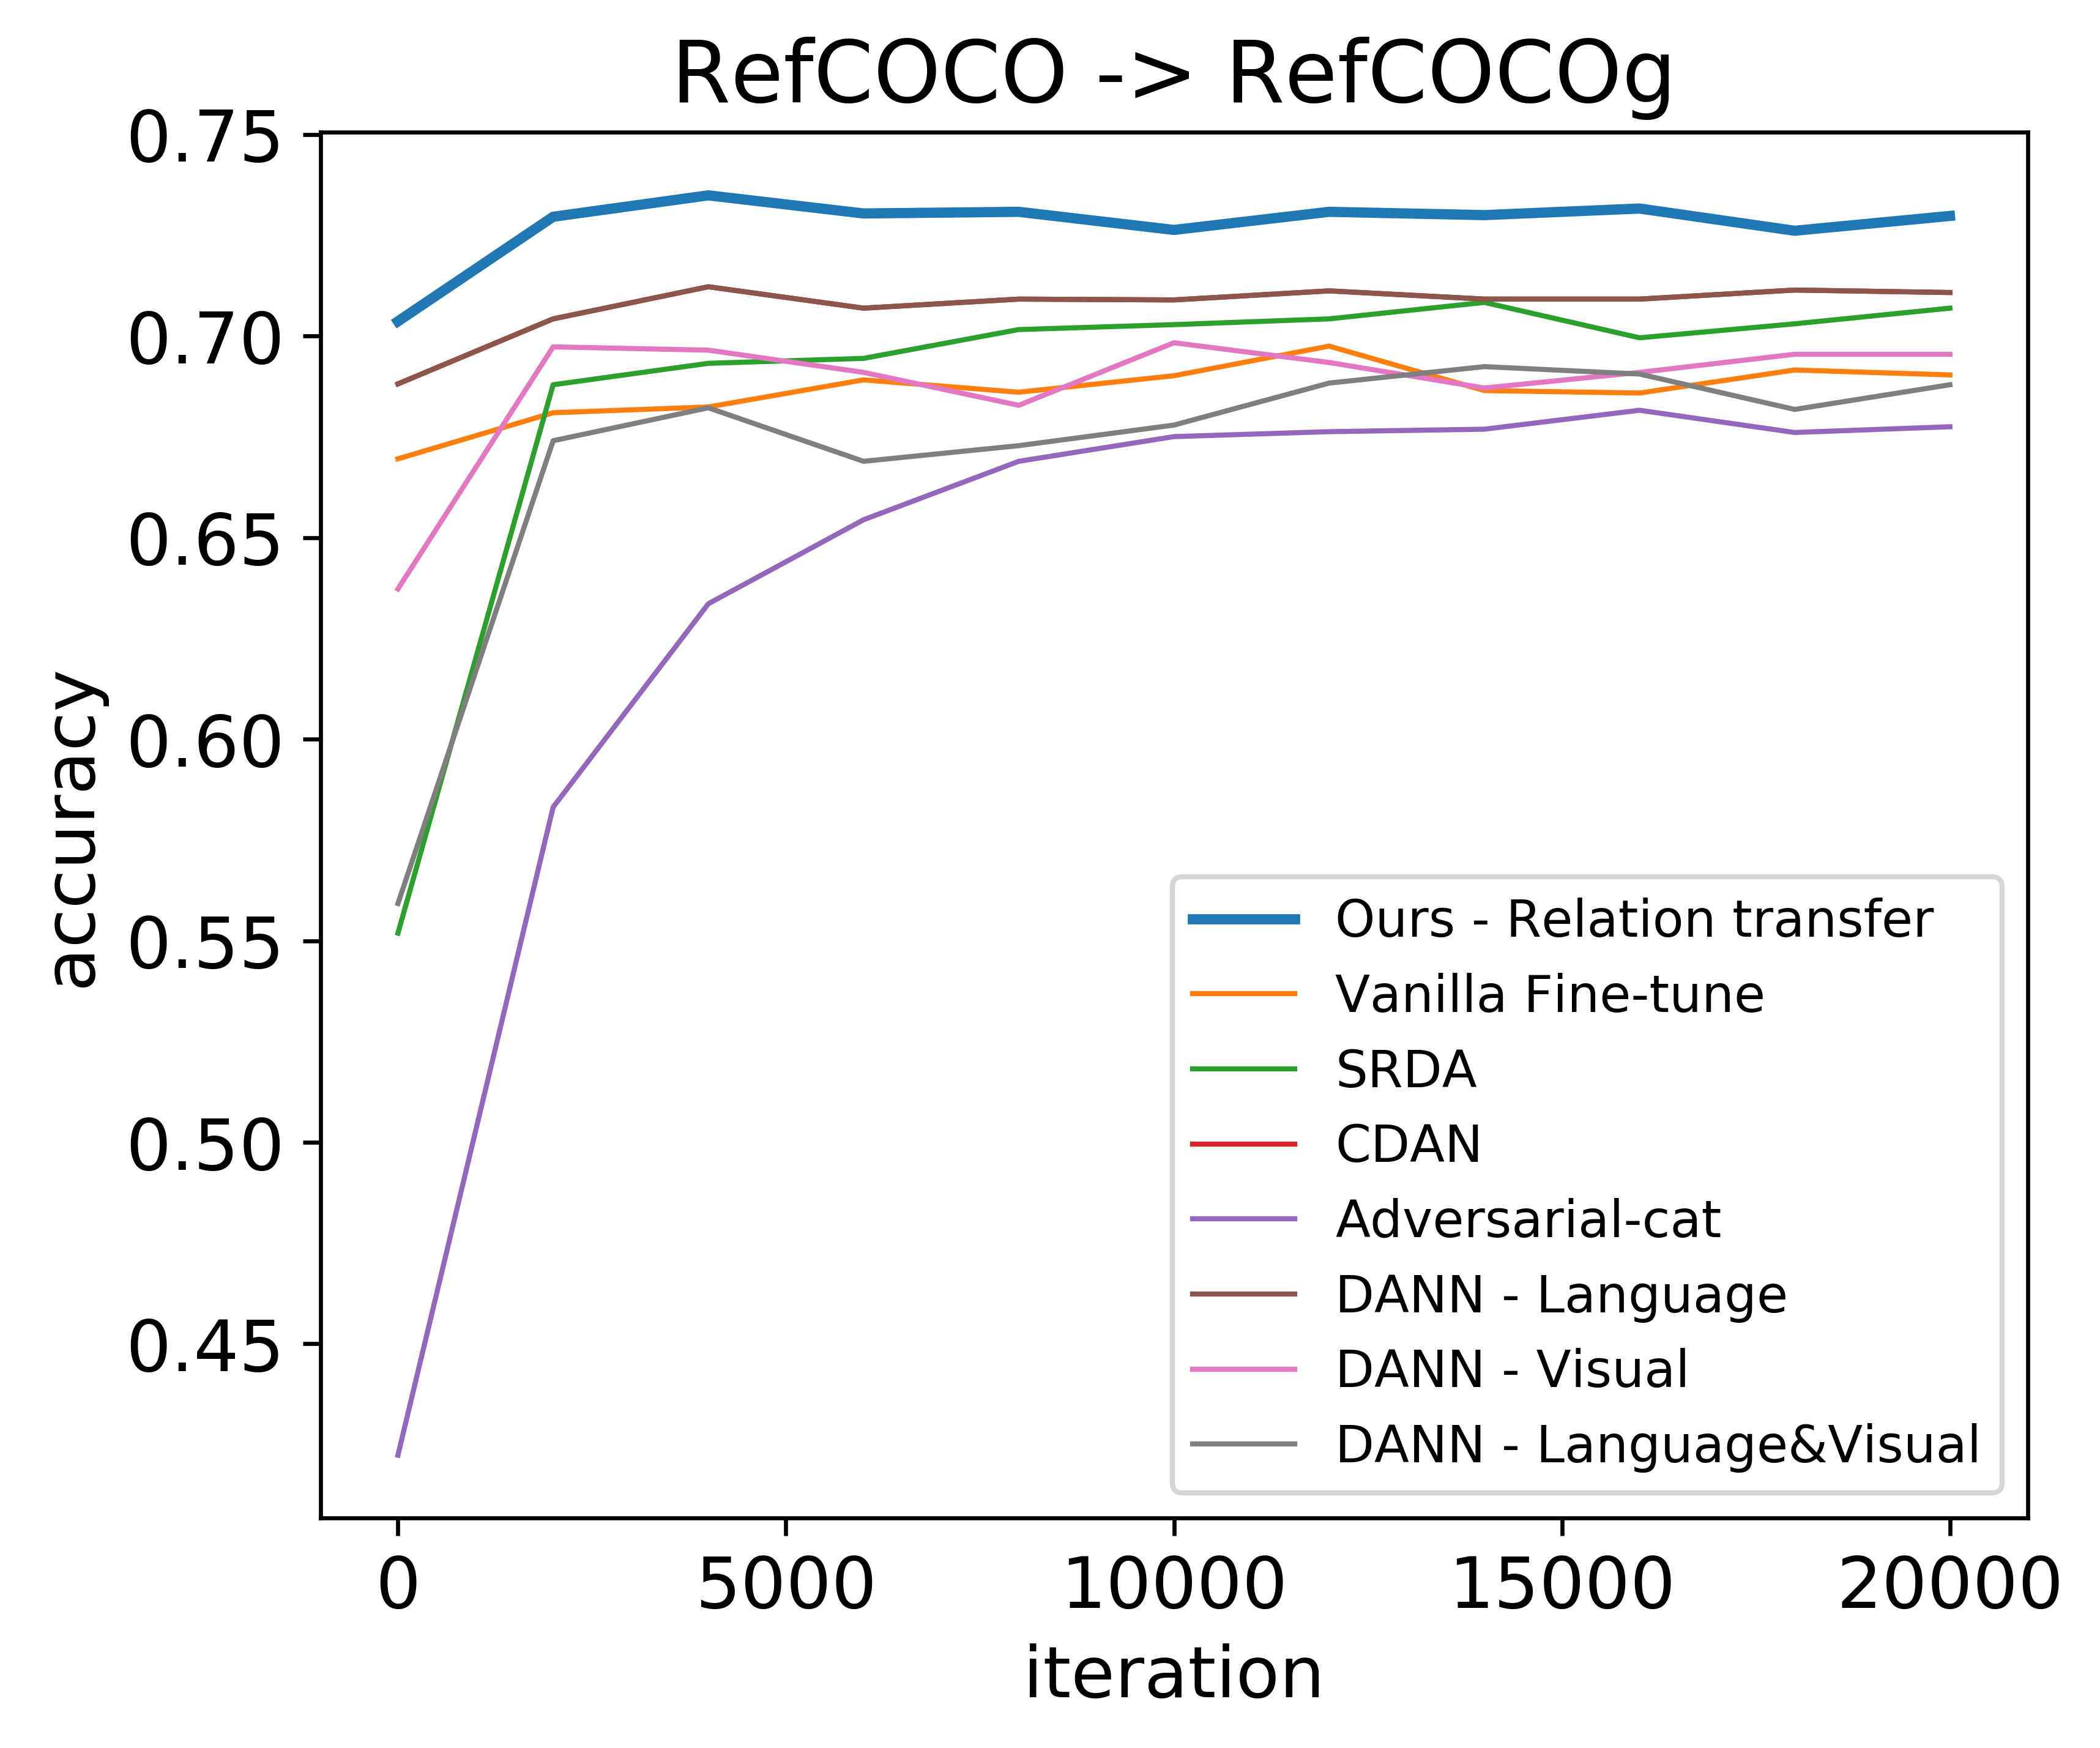}
\end{center}
   \caption{Convergence comparison of the proposed approach with baseline models for domain adaptation from RefCOCO to RefCOCOg }
\label{fig:refcocog}
\end{figure}

\begin{figure}[t]
\begin{center}
% \fbox{\rule{0pt}{2in} \rule{0.9\linewidth}{0pt}}
   \includegraphics[width=0.95\linewidth]{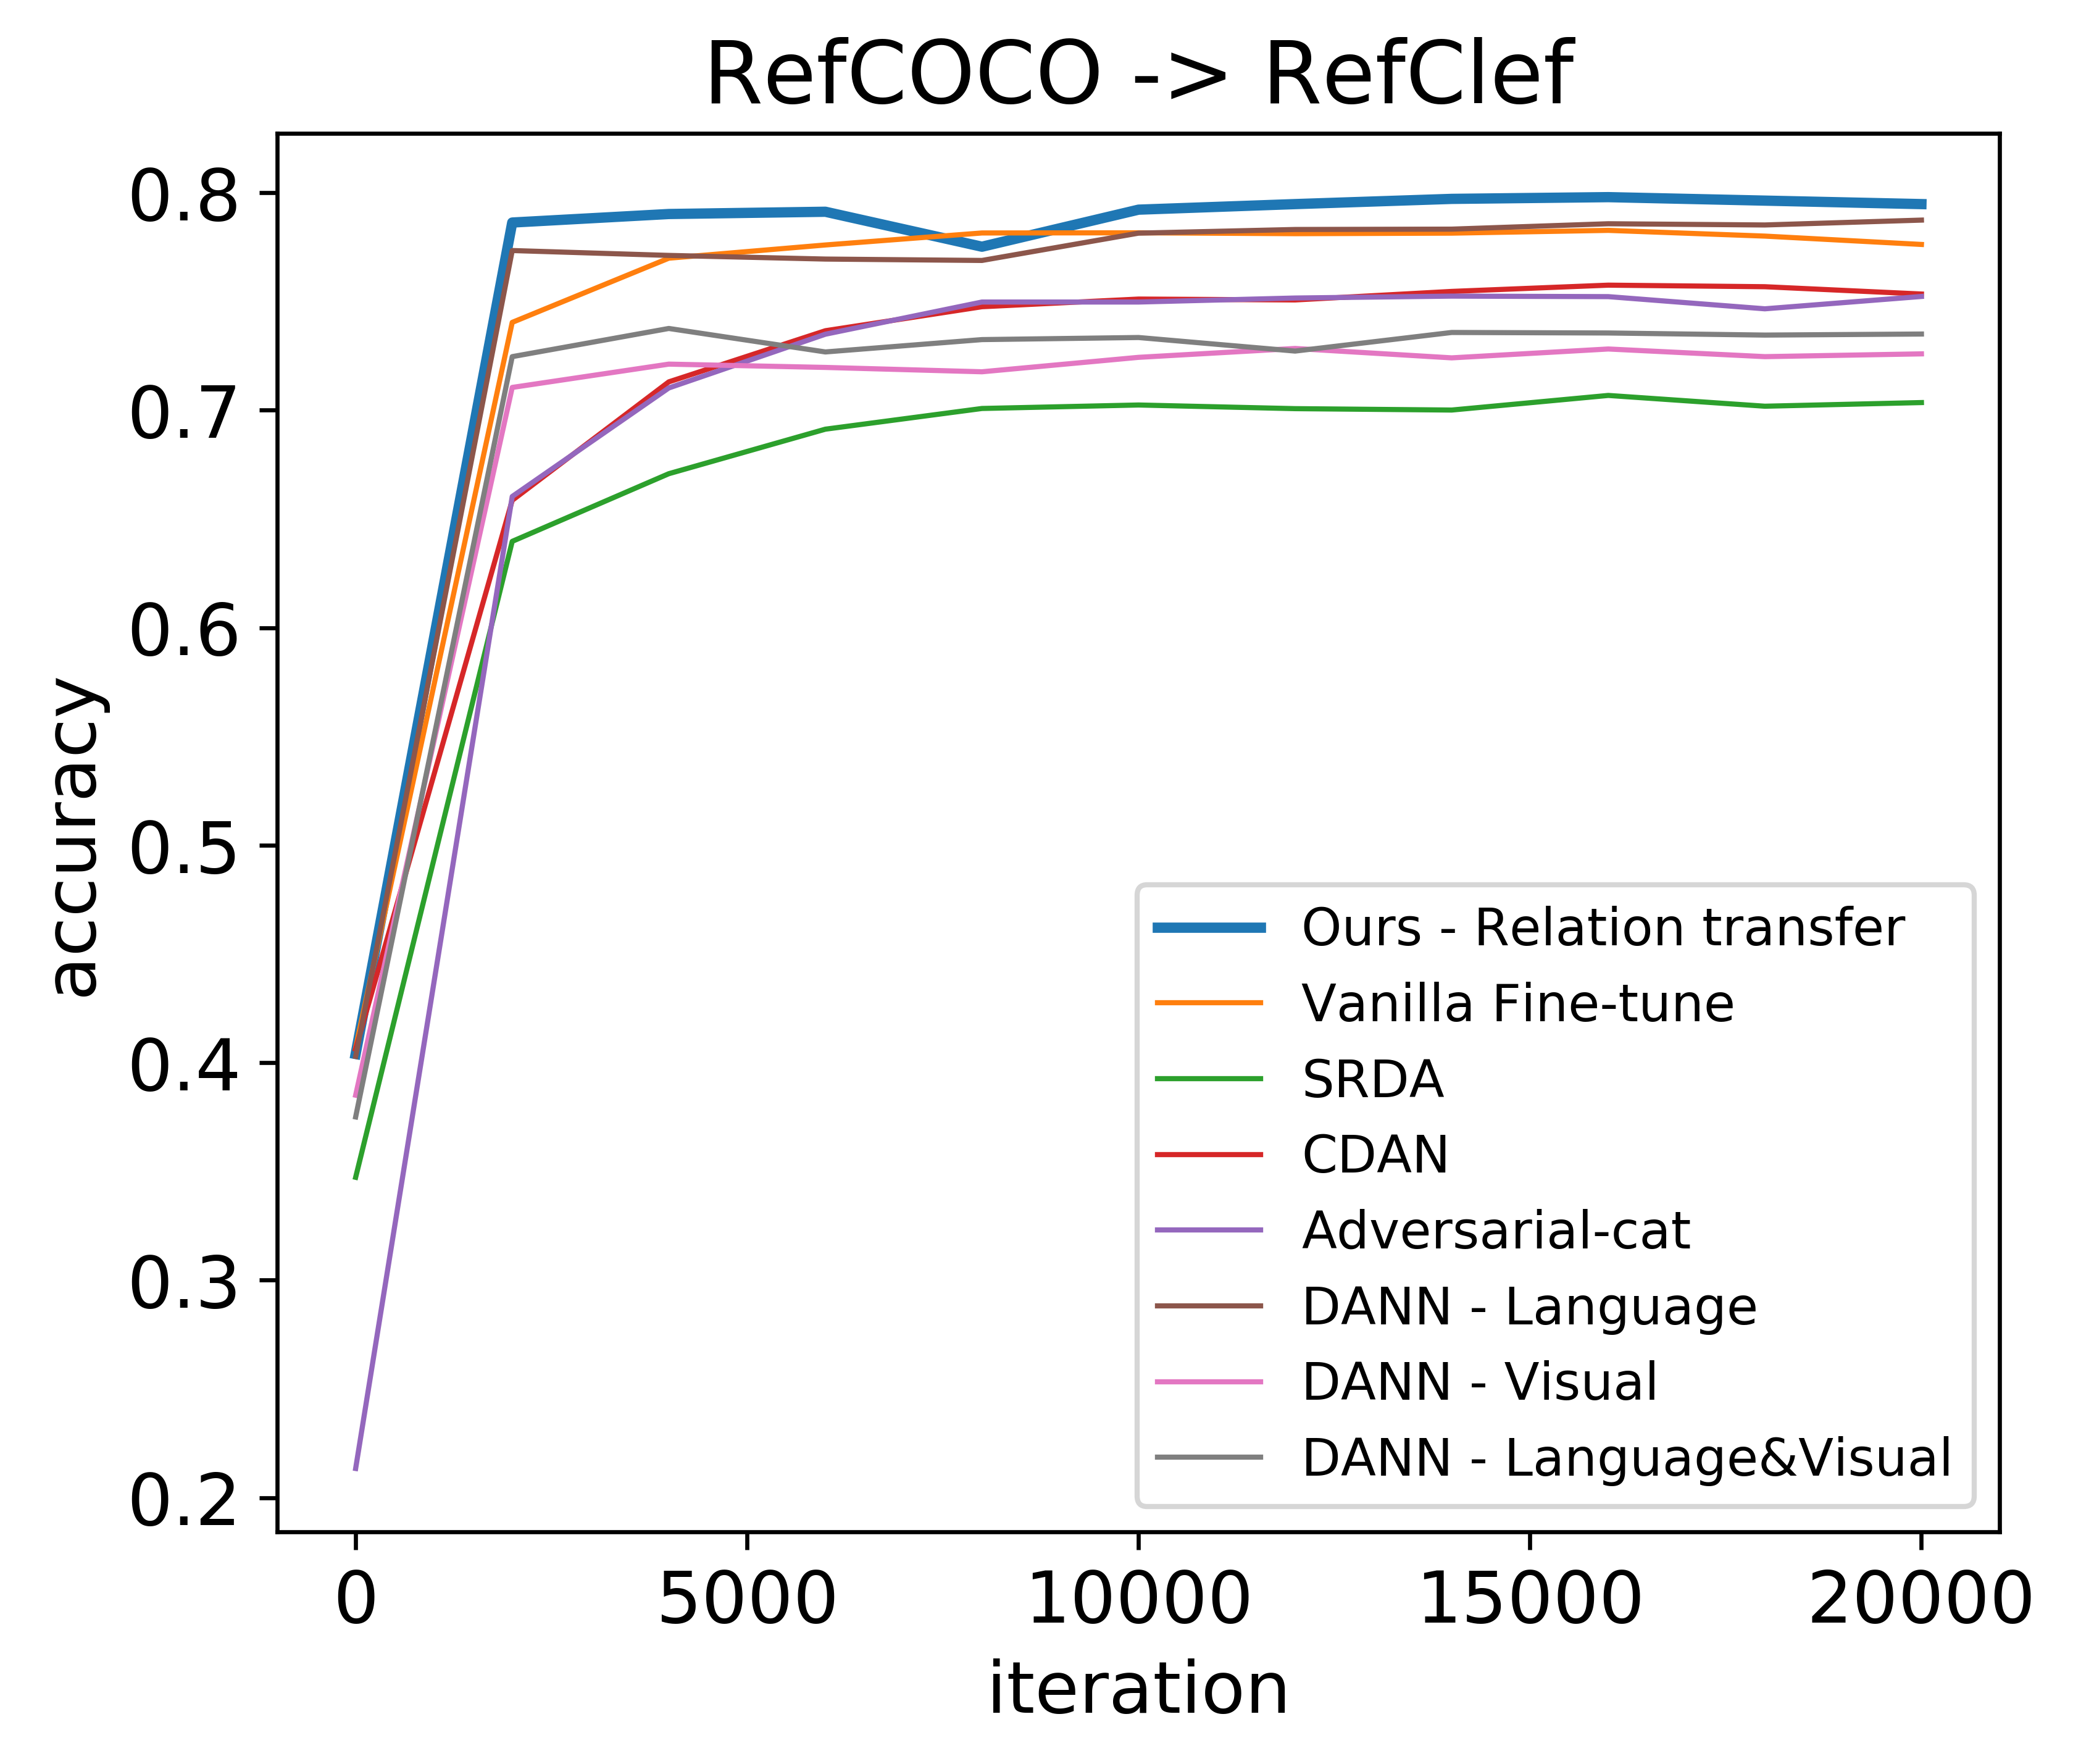}
\end{center}
   \caption{Convergence comparison of the proposed approach with baseline models for domain adaptation from RefCOCO to RefClef\ }
\label{fig:refclef}
\end{figure}

% Please add the following required packages to your document preamble:
% \usepackage[table,xcdraw]{xcolor}
% If you use beamer only pass "xcolor=table" option, i.e. \documentclass[xcolor=table]{beamer}

% \begin{table}[h]
% \centering
% \caption{Initial performance (Best results are \textbf{bolded})}
% \label{tab:suppl-swith}
% \begin{tabular}{l|ccc}
% \toprule
%   & RefCOCO+  & RefCOCOg &RefClef  \\
% \midrule\midrule
% Finetune on target & 0.354341                          & 0.40678237 & 0.66952614 \\
% DANN - Language~\cite{ganin2015unsupervised}          & 0.59537089                        & 0.40286331 & 0.68811275 \\
% DANN - Visual~\cite{ganin2015unsupervised}        & 0.36298569                        & 0.38502759 & 0.6372549 \\
% DANN - Language\&Visual~\cite{ganin2015unsupervised}          & 0.59881019                        & 0.37502999 & 0.55923203 \\
% Adversarial-cat \cite{tzeng2017adversarial}  &   0.3564789                         & 0.21338879 & 0.42238562  \\
% CDAN\cite{long2017conditional}               &  0.61042945                        & 0.40622251 & 0.68811275    \\
% SRDA\cite{cai2019learning}              & 0.528909                          & 0.34727665 & 0.55187908 \\
% Ours          &    0.63106525 & 0.40398304 & 0.70363562   \\
% \bottomrule
% \end{tabular}
% \end{table}
